# Supplementary material for: Relatively Complete Verification of Probabilistic Programs
Source: arXiv:2010.14548 source file (2022-01-28)
Supplement: Supplementary file 1 [file appendix_products.tex]

\subsection{Proof of Lemma~\ref{lem:aux_products_of_exp}}

\begin{proof}
	\label{proof:aux_products_of_exp}
	
	By induction on $i$ and Lemma~\ref{thm:prenex:aux}. \\ \\
	\noindent
	\emph{Base case $i=0$.} If $i = 0$, then $f_1$ is quantifier-free and the claim follows from applying the rules given in Lemma~\ref{thm:prenex-rules}. 
	Since $\FF_1$ and $\FF_2$ do not share logical variables, we can rename the bound variables back to $\VV_1, \ldots, \VV_i$.\\ \\
	\noindent
	\emph{Induction hypothesis.} Assume for some arbitrary, but fixed, $i \in \Nats$, that the lemma holds for all $\FF_1, \FF_2$, and $\FF$ of the required form. \\ \\
	\noindent
	\emph{Induction step.} Let 
	\begin{align*}
	\FF_1 &\eeq \Quant_1 \VV_1 \ldots \Quant_i \VV_i \colon \Quant_{i+1} \VV_{i+1} \colon \iverson{\BB_1} \\
	\FF_2 & \eeq  \Quant'_1 \VV'_1 \ldots \Quant'_j \VV'_j \colon \iverson{\BB_2}~.
	\end{align*}
	We distinguish the cases $\Quant_1 = \Sup$ and $\Quant_1 = \Inf$.
	Notice that $\sem{\FF_2}{\sigma}{\interpret} \in \{0,1\}$. For $\Quant_1 = \Sup$, we have
	\begin{align*}
	& \sem{\FF_1}{\sigma}{\interpret}
	\cdot \sem{\FF_2}{\sigma}{\interpret} \\
	\eeq & \sem{\Quant_1 \VV_1 \ldots \Quant_i \VV_i \colon \Quant_{i+1} \VV_{i+1} \colon \iverson{\BB_1}}{\sigma}{\interpret}
	\cdot \sem{\Quant'_1 \VV'_1 \ldots \Quant'_j \VV'_j \colon \iverson{\BB_2}}{\sigma}{\interpret} 
	\tag{by definition} \\
	\eeq & 
	\sup \setcomp{
		\sem{\Quant_2 \VV_2 \ldots  \Quant_{i+1} \VV_{i+1} \colon \iverson{\BB_1}}{\sigma}{\interpret\statesubst{\VV_1}{\RR}}    
	}{\RR \in \PosRats} \\
	& \quad \cdot \sem{\Quant'_1 \VV'_1 \ldots \Quant'_j \VV'_j \colon \iverson{\BB_2}}{\sigma}{\interpret} 
	\tag{by definition} \\
	\eeq & 
	\sup \setcomp{
		\sem{\Quant_2 \VV_2 \ldots  \Quant_{i+1} \VV_{i+1} \colon \iverson{\BB_1}}{\sigma}{\interpret\statesubst{\VV_1}{\RR}} 
		\cdot 
		\sem{\Quant'_1 \VV'_1 \ldots \Quant'_j \VV'_j \colon \iverson{\BB_2}}{\sigma}{\interpret} 
	}{\RR \in \PosRats} \\
	\tag{by Lemma~\ref{thm:prenex:aux} since $\sem{\FF_2}{\sigma}{\interpret} \in \{0,1\}$} \\
	\eeq & 
	\sup \setcomp{
		\sem{\Quant_2 \VV_2 \ldots  \Quant_{i+1} \VV_{i+1} \colon \iverson{\BB_1}}{\sigma}{\interpret\statesubst{\VV_1}{\RR}} 
		\cdot 
		\sem{\Quant'_1 \VV'_1 \ldots \Quant'_j \VV'_j \colon \iverson{\BB_2}}{\sigma}{\interpret\statesubst{\VV_1}{\RR}} 
	}{\RR \in \PosRats} \\
	\tag{$\VV_1$ does not occur in $\FF_2$ by assumption} \\
	\eeq & 
	\sup \setcomp{
		\sem{\Quant_2 \VV_2 \ldots  \Quant_{i+1} \VV_{i+1} \colon
			\Quant'_1 \VV'_1 \ldots \Quant'_j \VV'_j \colon
			\iverson{\BB_1} \cdot \iverson{\BB_2}}{\sigma}{\interpret\statesubst{\VV_1}{\RR}} 
	}{\RR \in \PosRats}
	\tag{by I.H.}  \\
	\eeq &\sem{\Quant_1 \VV_1 \colon \Quant_2 \VV_2 \ldots  \Quant_{i+1} \VV_{i+1} \colon
		\Quant'_1 \VV'_1 \ldots \Quant'_j \VV'_j \colon
		\iverson{\BB_1} \cdot \iverson{\BB_2}}{\sigma}{\interpret}~.
	\tag{by definition}
	\end{align*}

	The case $\Quant_1 = \Inf$ is completely analogous.

\end{proof}
