# Supplementary material for: Relatively Complete Verification of Probabilistic Programs
Source: arXiv:2010.14548 source file (2022-01-28)
Supplement: Supplementary file 2 [file appendix.tex]

\appendix
\newpage

\section{Appendix to Section~\ref{sec:normalforms} (Normal Forms)}

\input{appendix_normalforms}

%\section{Appendix to Section~\ref{sec:product_of_exp} (Products of Expectations)}
%\input{appendix_products}

\section{Appendix to Section~\ref{sec:embedding} (Embedding of FO Arithemtic)}

\input{appendix_embedding}

\section{Appendix to Section~\ref{sec:sums_prod_via_goedel} (Sums, Products, and Infinite Series of Syntactic Expectations via G\"odel)}

\input{appendix_sums_prod_via_goedel}

\section{Appendix to Section~\ref{sec:expressiveness} (Expressiveness of our Language)}
\input{appendix_expressiveness}
